# Supplementary material for: The paramagnetic Lyddane-Sachs-Teller relation
Source: arXiv:2405.15382 source file (2024-08-08)
Supplement: Supplementary file 1 [file PRL_supplementary__1_.pdf]

# Supplementary material to: The magnetic Lyddane-Sachs-Teller relation

Viktor Rindert,[1,*] Vanya Darakchieva,[1,2] Tapati Sarkar,[3] and Mathias Schubert[4,1]

[1]*NanoLund and Solid State Physics, Lund University, S-22100 Lund, Sweden*
[2]*Department of Physics, Chemistry, and Biology (IFM), Linköping University, SE 58183, Linköping, Sweden*
[3]*Department of Materials Science and Engineering, Uppsala University, Box 35, SE-751 03 Uppsala, Sweden.*
[4]*Department of Electrical and Computer Engineering, University of Nebraska-Lincoln, Lincoln, NE 68588, USA*
(Dated: May 24, 2024)

## I. 4×4 MATRIX FORMALISM FOR THZ MAGNETIC RESONANCE ELLIPSOMETRY

The data analyzed in the main manuscript is in the form of Mueller matrix elements. Mueller matrices $M$ are 4×4 matrices that transform Stokes vectors $\bar{S} = (I_x + I_y, I_x - I_y, I_{+45} - I_{-45}, I_R - I_L)^T$ where I is intensity, the subscripts denote different polarization settings, and $T$ is the transpose. For instance, the Mueller matrix of a sample $M_{Sample}$ represents how the polarization of the light changes upon reflection or transmission through the sample:

$$\bar{S}_{\text{out}} = M_{\text{Sample}} \bar{S}_{in}. \tag{1}$$

In this work, we measure the upper-left 3×3 submatrix using an in-house built THz ellipsometer. The (Berreman) 4×4 matrix method is utilized in this work to model calculate the Mueller matrices. The 4×4 matrix method is derived from Maxwell's equations matrix form:[1]

$$\frac{\partial \Psi}{\partial z} = i\frac{\omega}{c}\Delta_B \Psi, \tag{2}$$

where $\omega$ is the frequency of the incident light, $c$ the speed of light, $z$ the direction of the sample surface normal, $\Psi = (E_x, E_y, H_x, H_y)^T$ where $E$ and $H$ are the electric and magnetic component of the electromagnetic wave, respectively, and

$$\Delta_B = \begin{pmatrix} -q_x\frac{\varepsilon_{zx}}{\varepsilon_{zz}} & q_x(-\frac{\varepsilon_{zy}}{\varepsilon_{zz}} + \frac{\mu_{zx}}{\mu_{zz}}) & \mu_{yx} - \frac{\mu_{yz}\mu_{zx}}{\mu_{zz}} & -q_x^2\frac{1}{\varepsilon_{zz}} + \mu_{yy} - \frac{\mu_{yz}\mu_{zy}}{\mu_{zz}} \\ 0 & -q_x\frac{\mu_{xz}}{\mu_{zz}} & -\mu_{xx} + \frac{\mu_{xz}\mu_{zx}}{\mu_{zz}} & -\mu_{xy} + \frac{\mu_{xz}\mu_{zy}}{\mu_{zz}} \\ -\varepsilon_{yx} + \frac{\varepsilon_{yz}\varepsilon_{zx}}{\varepsilon_{zz}} & -\varepsilon_{yy} + \frac{\varepsilon_{yz}\varepsilon_{zy}}{\varepsilon_{zz}} + q_x^2\frac{1}{\mu_{zz}} & -q_x\frac{\mu_{zx}}{\mu_{zz}} & q_x(\frac{\varepsilon_{yz}}{\varepsilon_{zz}} - \frac{\mu_{zy}}{\mu_{zz}}) \\ \varepsilon_{xx} - \frac{\varepsilon_{xz}\varepsilon_{zx}}{\varepsilon_{zz}} & \varepsilon_{xy} - \frac{\varepsilon_{xz}\varepsilon_{zy}}{\varepsilon_{zz}} & 0 & -q_x\frac{\varepsilon_{xz}}{\varepsilon_{zz}} \end{pmatrix}, \tag{3}$$

where $q_x = n_I \sin\theta$ is the $x$-component of the reduced wavevector $\frac{\omega}{c}\mathbf{q} = \mathbf{k}$, and $\theta$ is the angle of incidence. Knowing the dielectric ($\varepsilon$) and permeability tensor ($\mu$) elements and thus the $\Delta_B$-matrix is instrumental to calculate the Mueller matrix of the sample. The calculation of $M_{\text{Sample}}$ for a sample with one or multiple layers follows by calculating the transfer matrix $L_j$ for each layers:

$$L_j = \exp\left(-i\frac{\omega}{c}\Delta_B d\right), \tag{4}$$

where $d$ is the thickness of the layer, together with the incident matrix (assuming ambient air as incident medium)

$$L_R^{-1} = \frac{1}{2}\begin{pmatrix} 0 & 1 & -(\cos\theta)^{-1} & 0 \\ 0 & 1 & (\cos\theta)^{-1} & 0 \\ (\cos\theta)^{-1} & 0 & 0 & 1 \\ -(\cos\theta)^{-1} & 0 & 0 & 1 \end{pmatrix}, \tag{5}$$

and exit matrix

$$L_T = \begin{pmatrix} 0 & 0 & \cos(\Phi_T) & \cos(\Phi_T) \\ 1 & 1 & 0 & 0 \\ -n_T\cos(\Phi_T) & n_T\cos(\Phi_T) & 0 & 0 \\ 0 & 0 & n_T & n_T \end{pmatrix}, \tag{6}$$

where $\cos(\Phi_T) = \sqrt{1 - (1/n_T^2 \sin^2(\theta)}$. The total transfer matrix $L$ is then calculated

$$L = L_R^{-1} \left( L_1 L_2 \ldots L_N \right) L_T, \tag{7}$$

where $N$ is the number of layers. The Mueller-matrix elements $M_{23}$ and $M_{32}$ are then calculated with the expressions

$$M_{23} = \Re\left( \frac{(L_{11}L_{43} - L_{13}L_{41})(L_{11}L_{23} - L_{13}L_{21})^*}{L_{11}L_{33} - L_{13}L_{31}} - \frac{(L_{33}L_{21} - L_{31}L_{23})(L_{33}L_{41} - L_{31}L_{43})^*}{L_{11}L_{33} - L_{13}L_{31}} \right), \tag{8}$$

$$M_{32} = \Re\left( \frac{(L_{11}L_{43} - L_{13}L_{41})(L_{33}L_{41} - L_{31}L_{43})^*}{L_{11}L_{33} - L_{13}L_{31}} - \frac{(L_{33}L_{21} - L_{31}L_{23})(L_{11}L_{23} - L_{13}L_{21})^*}{L_{11}L_{33} - L_{13}L_{31}} \right), \tag{9}$$

where $*$ symbolizes the complex conjugate. These elements show significant features in the Mueller matrix that can be measured with our THz ellipsometer. An optimization procedure is used to obtain the optimized permeability tensor. The following unbiased least-squares sum is minimized

$$S = \sum_{i=1}^{j} (y_i - f_i)^2, \tag{10}$$

where the $y_i$'s are the experimentally obtained effective Mueller matrix elements, and $f_i$ are the calculated effective Mueller matrix elements. Specifically, we use effective Mueller matrix elements because $M_{23} = M_{32}$ by observation from experiment as well as due to the model permeability tensor used in this work. Hence, for convenience, we use the effective Mueller-matrix element

$$M_{23,32} = \frac{M_{23} + M_{32}}{2}. \tag{11}$$

The analysis of $M_{23,32}$ is then sufficient to determine frequencies, amplitudes, and relaxation times parameters using the permeability model tensor. However, the thickness of the sample also needs to be determined.

## II. SAMPLE THICKNESS DETERMINATION

For a measurement performed at single temperature and magnetic field, thickness and model permeability parameters are highly correlated. This can be seen in Fig. 1. Here, the best-match model calculated dc magnetic susceptibility $\chi_0$ is shown versus the thickness of the sample in the model when the thickness parameter is fixed. The apparent dependence of the magnetization on the thickness parameter is akin to the index of refraction and thickness correlation in thin film often observed in ellipsometry. A way out is to reduce parameter correlation by use of parametric response model functions.

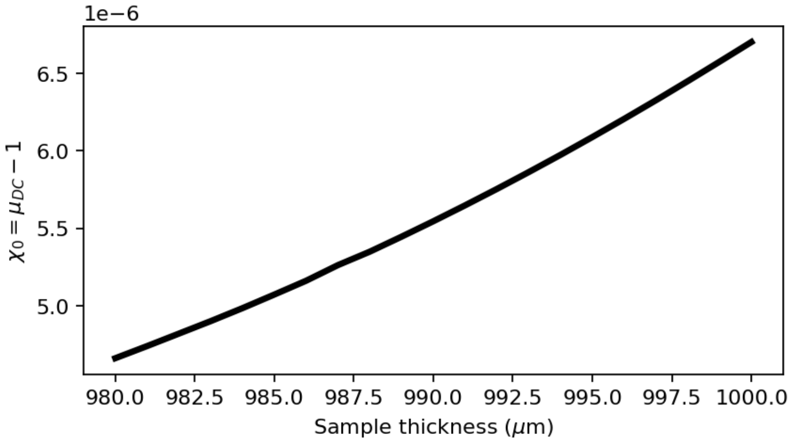


FIG. 1. Calculated dc magnetic susceptibility as a function of the assumed sample thickness $d$ in the data analysis using the model outlined in the main text.

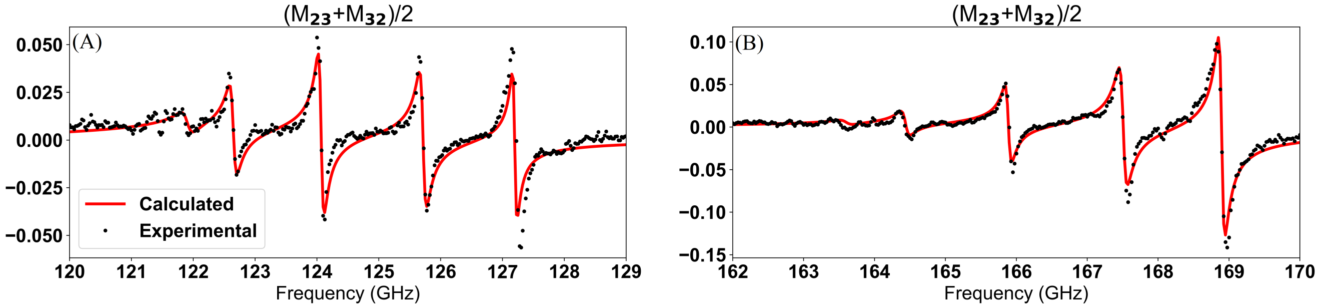


FIG. 2. Experimental data (black dots) obtained by THz EPR ellipsometry and best-match model (red line) obtained from the Bloch-Brillouin model detailed in the text. In (A), a spectroscopic scan at 4.42 T is shown, and in (B) at 5.91 T. Both scans were performed at 15 K.

We break the correlation between the dc and thickness parameters by analysing measurements taken at two different magnetic field, $B = 4.42$ T and $B = 5.91$ T and constant temperature. To put further constraints on the model analysis, we employed the Bloch-Brillouin model, as detailed in Ref. 2. This combined analysis results in independent determination of thickness and permeability model parameters. The Bloch-Brillouin model dictates the following amplitude distribution which depends on temperature and magnetic field:

$$M_0 = \sum_j^5 M_{0,j}, \tag{12}$$

$$M_0 = \frac{g\mu_B}{2}(5(n_{+5/2} - n_{+3/2}) + 8(n_{+3/2} - n_{+1/2}) + 9(n_{+1/2} - n_{-1/2}) + 8(n_{-1/2} - n_{-3/2}) + 5(n_{-3/2} - n_{-5/2})), \tag{13}$$

where the population differences are given by normalized Boltzmann factors:

$$n_n - n_{n-1} = \frac{e^{-E_n/kT} - e^{-E_{n-1}/kT}}{\sum_j e^{-E_j/kT}} n_e. \tag{14}$$

and the magnetic susceptibility is

$$\chi_0 = \frac{M_0}{B_0} = \sum_j^5 \frac{M_{0,j}}{B_0} = \sum_j^5 \chi_{0,j}. \tag{15}$$

The magnetic susceptibility values are then inserted into the permeability tensor

$$\boldsymbol{\mu_M} = \mathbf{1} + \sum_{j=1}^5 \begin{pmatrix} \frac{\chi_{0,j}\omega_{0,j}^2}{\omega_{0,j}^2 - \omega^2 - 2i\omega/T_2} & -i\frac{\chi_{0,j}\omega_{0,j}\omega}{\omega_{0,j}^2 - \omega^2 - 2i\omega/T_2} & 0 \\ i\frac{\chi_{0,j}\omega_{0,j}\omega}{\omega_{0,j}^2 - \omega^2 - 2i\omega/T_2} & \frac{\chi_{0,j}\omega_{0,j}^2}{\omega_{0,j}^2 - \omega^2 - 2i\omega/T_2} & 0 \\ 0 & 0 & \chi_0 \end{pmatrix}, \tag{16}$$

which in turn is inserted into (3) to perform model analysis. The thereby obtained best-match model calculated thickness parameter was determined to be $d = (989 \pm 2)$ $\mu$m within a 95% confidence interval. The comparison between the best-match model and experimental data is shown in Fig. 2. Assuming that the thickness parameter is the most significant cause of the uncertainty thus gives us an error estimate of the calculated dc permeability which can be written as

$$\mu_{\text{dc}} = 1 + (5.4 \pm 0.2) \cdot 10^{-6} \tag{17}$$

## III. CALCULATION OF SQUID DC PERMEABILITY AT $B\angle(0001) = 45^\circ$

To accurately extrapolate the DC magnetization to a magnetic field direction of 45° relative to the Gallium Nitride c-axis, it is essential to consider the variations in the distribution of magnetic moments with changes in the magnetic

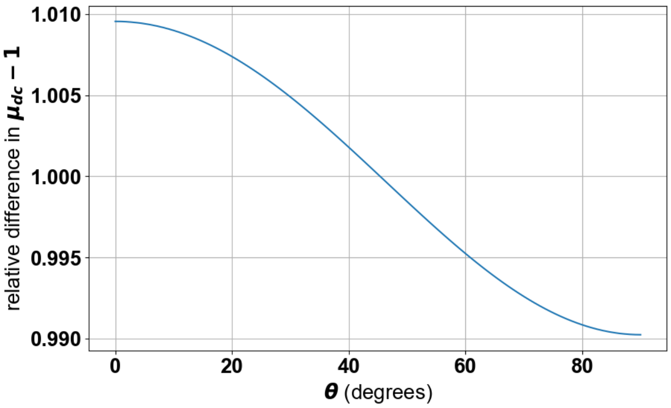


FIG. 3. Calculated $\chi_0 = \mu_{\mathrm{dc}} - 1$ as a function of the angle between the magnetic field and the c-axis, normalized such that $\mu_{dc}(\theta = 45^\circ) - 1 = 1$, demonstrating an expected variation of around 1% from the $\theta = 45^\circ$ case due to changes in magnetic field orientation, using parameters reported by Kashiwagi et al[4].

field direction. This can be effectively modeled using the spin-Hamiltonian described by Geschwind et al.[3]:

$$\begin{aligned}\mathcal{H} = {} & g_{||}\mu_B B_0 S_z \cos\theta + \frac{1}{2} g_\perp \mu_B B_0 \sin\theta (S_+ + S_-) + D(S_z^2 - \frac{1}{3}S(S+1)) \\ & - \frac{1}{180}(a - F)(35S_z^4 - 30S(S+1)S_z^2 + 25S_z^2 - 6S(S+1) + 3S^2(S+1)^2) \\ & + \frac{\sqrt{2}}{36} a(S_z(S_+^3 e^{-i3(\psi\pm\alpha)} + S_-^3 e^{i3(\psi\pm\alpha)}) + (S_+^3 e^{-i3(\psi\pm\alpha)} + S_-^3 e^{i3(\psi\pm\alpha)})S_z),\end{aligned} \tag{18}$$

where $\theta$ is the angle between the magnetic field and the c-axis. The parameters $g_{||}$ and $g_\perp$ represent the parallel and perpendicular Zeeman splitting factors, respectively, while $D$, $a$, and $F$ are zero-field splitting parameters. The spin operators $S_z$, $S_+$, $S_-$, and $S$ denote the conventional $S = 5/2$ spin components. The angles $\psi = \pi/6$ and $\alpha = \pi/6$ define the orientations relative to the crystallographic axes.

Utilizing the spin Hamiltonian parameters from Kashiwagi et al.[4], where $D = -2300$ MHz, $a = 240$ MHz, $F = -27$ MHz, $g_{||} = 2.007$, and $g_\perp = 2.009$ were reported, we calculate the new population differences using Eq. (14) and the magnetization using the population differences in Eq. (13). Figure 3 illustrates the computed magnetization as a function of the angle $\theta$, highlighting an expected variation of approximately 1% of the magnetic dc susceptibility when the magnetic field direction is in-plane compared to when $\theta = 45^\circ$.

---

[*] Electronic mail: viktor.rindert@ftf.lth.se
[1] "Principles of optics," in *Spectroscopic Ellipsometry* (John Wiley & Sons, Ltd, 2007) Chap. 2, 3, 4, pp. 13–207.
[2] V. Rindert, S. Richter, A. Ruder, V. Darakchieva, and M. Schubert, Phys. Rev. B **XXX**, X (2024).
[3] S. Geschwind, Phys. Rev. **121**, 363 (1961).
[4] T. Kashiwagi, S. Sonoda, H. Yashiro, Y. Ishihara, A. Usui, Y. Akasaka, and M. Hagiwara, Japanese Journal of Applied Physics **46**, 581 (2007).
